# Supplementary material for: Few-Shot Learning for Opinion Summarization
Source: arXiv:2004.14884 source file (2020-10-10)
Supplement: Supplementary file 3 [file mt_summary_instructions.tex]

\subsection{AMT Summary Writing Instructions}
\label{sec:amt_summ_instr}
